# Supplementary material for: Personalized Schedules for Surveillance of Low Risk Prostate Cancer Patients
Source: arXiv:1711.00285 source file (2017-11-01)
Supplement: Supplementary file 2 [file derivation_estimation_mean_var.tex]

% !TEX root =  ../supplementary.tex
\section{Derivations for Equation \ref{eq : expected_time_survprob} and \ref{eq : var_time_survprob} of the Main Manuscript}
In this section we present the derivations for Equation \ref{eq : expected_time_survprob} and \ref{eq : var_time_survprob} of the main manuscript. To this end, we first expand the formula for dynamic survival probability presented in Equation \ref{eq : dynamic_surv_prob} of the main manuscript.
\begin{equation}
\label{eq : dyn_surv_prob_expanded}
\begin{split}
\pi_j(u \mid t, s) &= \mbox{Pr}\big\{T^*_j \geq u \mid  T^*_j >t, \mathcal{Y}_j(s\big), D_n)\\
&= \int \int \mbox{Pr}\big(T^*_j \geq u \mid  T^*_j >t, \bmath{b}_j,\bmath{\theta}\big) p\big\{\bmath{b}_j \mid T^*_j>t, \mathcal{Y}_j(s), \bmath{\theta}\big\} p(\bmath{\theta} \mid \mathcal{D}_n) \rmn{d} \bmath{b}_j \rmn{d} \bmath{\theta}\\
&= \int \int \frac{\exp\big\{-H_j(u | \bmath{b}_j, \bmath{\theta})\big\}}{\exp\big\{-H_j(t | \bmath{b}_j, \bmath{\theta})\big\}} p\big\{\bmath{b}_j \mid T^*_j>t, \mathcal{Y}_j(s), \bmath{\theta}\big\} p(\bmath{\theta} \mid \mathcal{D}_n) \rmn{d} \bmath{b}_j \rmn{d} \bmath{\theta},
\end{split}
\end{equation}
where $H_j(u | \bmath{b}_j, \bmath{\theta}) = \int_0^u h_i(s \mid \bmath{b}_j, \bmath{\theta}\big)\rmn{d} s$ is the cumulative hazard up to time point $u$.

\subsection{Derivation of Equation \ref{eq : expected_time_survprob} of the Main Manuscript}
\begin{equation*}
E_g(T^*_j) = \int_t^{\infty} T^*_j g(T^*_j)\rmn{d} T^*_j.
\end{equation*}

Using integration by parts, wherein ${\rmn{d} \big\{-\pi_j(T^*_j \mid t, s)\big\}}/{\rmn{d} T^*_j} = g(T^*_j)$,
\begin{equation*}
\begin{split}
E_g(T^*_j) &= \Big[-T^*_j\pi_j(T^*_j \mid t, s)\Big]_t^\infty + \int_t^{\infty} \pi_j(T^*_j \mid t, s) \frac{\rmn{d} (T^*_j)}{\rmn{d} T^*_j} \rmn{d} T^*_j\\
&= t \pi_j(t \mid t, s) - \lim_{T^*_j\to \infty}T^*_j \pi_j(T^*_j \mid t, s) \\ & \quad + \int_t^{\infty} \pi_j(T^*_j \mid t, s) \rmn{d} T^*_j,
\end{split}
\end{equation*}
where $\pi_j(t \mid t, s) = \mbox{Pr}\big\{T^*_j \geq t \mid  T^*_j >t, \mathcal{Y}_j(s), D_n\big\} = 1$. As for $\lim_{T^*_j\to \infty}T^*_j \pi_j(T^*_j \mid t, s)$, the limit can be interchanged with the integral in Equation \ref{eq : dyn_surv_prob_expanded}, because as $T^*_j\to \infty$ the integrand in the equation converges uniformly on the domain of $(\bmath{b}_j, \bmath{\theta}\big)$. Thus,
\begin{equation*}
\begin{split}
\lim_{T^*_j\to \infty}T^*_j \pi_j(T^*_j \mid t, s) &=  \int \int \lim_{T^*_j\to \infty} \frac{T^*_j}{\exp\big\{H_j(T^*_j | \bmath{b}_j, \bmath{\theta})\big\}} \\ & \quad \times \frac{p\big\{\bmath{b}_j \mid T^*_j>t, \mathcal{Y}_j(s), \bmath{\theta}\big\} p(\bmath{\theta} \mid \mathcal{D}_n)}{\exp\big\{-H_j(t | \bmath{b}_j, \bmath{\theta})\big\}}  \rmn{d} \bmath{b}_j \rmn{d} \bmath{\theta}.\end{split}
\end{equation*}

Using L'Hospital's rule,
\begin{equation*}
\begin{split}
\lim_{T^*_j\to \infty}T^*_j \pi_j(T^*_j \mid t, s) &=  \int \int \frac{1}{\lim_{T^*_j\to \infty} \exp\big\{H_j(T^*_j | \bmath{b}_j, \bmath{\theta})\big\}H'_j(T^*_j | \bmath{b}_j, \bmath{\theta})} \\ & \quad \times \frac{p\big\{\bmath{b}_j \mid T^*_j>t, \mathcal{Y}_j(s), \bmath{\theta}\big\}p(\bmath{\theta} \mid \mathcal{D}_n)}{\exp\big\{-H_j(t | \bmath{b}_j, \bmath{\theta})\big\}} \rmn{d} \bmath{b}_j \rmn{d} \bmath{\theta}\\
&= \int \int 0 \times \frac{p\big\{\bmath{b}_j \mid T^*_j>t, \mathcal{Y}_j(s), \bmath{\theta}\big\}p(\bmath{\theta} \mid \mathcal{D}_n)}{\exp\big\{-H_j(t | \bmath{b}_j, \bmath{\theta})\big\}}  \rmn{d} \bmath{b}_j \rmn{d} \bmath{\theta}\\
&= 0.
\end{split}
\end{equation*}

In light of these results, we obtain:
\begin{equation*}
E_g(T^*_j) = t + \int_t^{\infty} \pi_j(T^*_j \mid t, s) \rmn{d} T^*_j.
\end{equation*}

\subsection{Derivation of Equation \ref{eq : var_time_survprob} of the Main Manuscript}
Since $\mbox{var}_g(T^*_j) = E_g\{(T^*_j)^2\} - E_g(T^*_j)^2$, we first show the derivation for $E_g\{(T^*_j)^2\}$.
\begin{equation*}
E_g\{(T^*_j)^2\} = \int_t^{\infty} (T^*_j)^2 g(T^*_j)\rmn{d} T^*_j.
\end{equation*}

Using integration by parts, wherein ${\rmn{d} \big\{-\pi_j(T^*_j \mid t, s)\big\}}/{\rmn{d} T^*_j} = g(T^*_j)$,
\begin{equation*}
\begin{split}
E_g\big\{(T^*_j)^2\big\} &= \Big[-(T^*_j)^2\pi_j(T^*_j \mid t, s)\Big]_t^\infty + \int_t^{\infty} \pi_j(T^*_j \mid t, s) \frac{\rmn{d} (T^*_j)^2}{\rmn{d} T^*_j} \rmn{d} T^*_j\\
&= t^2 \pi_j(t \mid t, s) - \lim_{T^*_j\to \infty}(T^*_j)^2 \pi_j(T^*_j \mid t, s) \\& \quad + 2 \int_t^{\infty} T^*_j \pi_j(T^*_j \mid t, s) \rmn{d} T^*_j\\
&= t^2 + 2 \int_t^{\infty} T^*_j \pi_j(T^*_j \mid t, s) \rmn{d} T^*_j.
\end{split}
\end{equation*}

Therefore,
\begin{equation*}
\begin{split}
\mbox{var}_g(T^*_j) &= t^2 + 2 \int_t^{\infty} T^*_j \pi_j(T^*_j \mid t, s) \rmn{d} T^*_j \\ & \quad - \bigg[t^2 +  \Big\{\int_t^\infty \pi_j(T^*_j \mid t, s) \rmn{d} T^*_j \Big\}^2 + 2t\int_t^\infty \pi_j(T^*_j \mid t, s) \rmn{d} T^*_j \bigg]\\
&=2 \int_t^{\infty} (T^*_j - t) \pi_j(T^*_j \mid t, s) \rmn{d} T^*_j -  \Big\{\int_t^\infty \pi_j(T^*_j \mid t, s) \rmn{d} T^*_j \Big\}^2.
\end{split}
\end{equation*}
