# Supplementary material for: Personalized Schedules for Surveillance of Low Risk Prostate Cancer Patients
Source: arXiv:1711.00285 source file (2017-11-01)
Supplement: Supplementary file 6 [file sim_study_graphs.tex]

% !TEX root =  ../supplementary.tex
\section{Simulation Study}
\subsection{Simulation Results for Dynamic Risk of GR Based Approach With a Fixed $\kappa = 0.95$}
In the main manuscript, for the personalized schedules based on dynamic risk of GR we chose $\kappa$ on the basis of $\mbox{F}_1$ score. However while conducting the simulation study, we also tried a fixed $\kappa$ of 0.95, which means that the next biopsy is scheduled at a time point where the dynamic risk of GR is 5\%. The results for this approach are presented in \ref{table : sim_study_pooled_estimates_extended}. In the table, the abbreviation Dyn. risk GR ($\mbox{F}_1$ score) corresponds to personalized schedules based on dynamic risk of GR based approach, with $\kappa$ chosen on the basis of $\mbox{F}_1$ score. The abbreviation Hybrid ($\mbox{F}_1$ score) corresponds to the hybrid approach between median time of GR and dynamic risk of GR ($\kappa$ chosen on the basis of $\mbox{F}_1$ score).

\begin{table}[!htb]
\caption{Estimated mean and standard deviation of the number of biopsies and offset (months).}
\label{table : sim_study_pooled_estimates_extended}
\begin{tabular}{lrrrr}
\Hline
\multicolumn{5}{c}{a) All subgroups}\\
\hline
Schedule          & $E(N^S_j)$ & $E(O^S_j)$ & ${\mbox{SD}(N^S_j)}$ & ${\mbox{SD}(O^S_j)}$ \\
\hline
Annual         & 5.24            & 6.01                & 2.53          & 3.46              \\
PRIAS          & 4.90            & 7.71                & 2.36          & 6.31\\
Dyn. risk GR ($\mbox{F}_1$ score)       & 4.69            & 6.66                & 2.19           & 4.38              \\
Hybrid ($\mbox{F}_1$ score)      & 3.75            & 9.70                & 1.71          & 7.25              \\
Dyn. risk GR ($\kappa=0.95$) & 5.15 & 6.02 & 2.51 & 3.47\\
Med. GR time & 2.06            & 13.88               & 1.41          & 11.80              \\
Exp. GR time & 1.92            & 15.08               & 1.19          & 12.11             \\
\hline
\multicolumn{5}{c}{b) Subgroup $G_1$}\\
\hline
Schedule        & $E(N^S_j)$ & $E(O^S_j)$ & ${\mbox{SD}(N^S_j)}$ & ${\mbox{SD}(O^S_j)}$ \\
\hline
Annual         & 4.32            & 6.02                & 3.13          & 3.44              \\
PRIAS          & 4.07            & 7.44                & 2.88          & 6.11    \\
Dyn. risk GR ($\mbox{F}_1$ score)       & 3.85            & 6.75                & 2.69          & 4.44              \\
Hybrid ($\mbox{F}_1$ score)       & 3.25            & 10.25               & 2.16          & 8.07              \\
Dyn. risk GR ($\kappa=0.95$) & 4.23 & 6.05 & 3.10 & 3.46\\
Med. GR time & 1.84            & 20.66               & 1.76          & 14.62             \\
Exp. GR time & 1.72            & 21.65               & 1.47          & 14.75             \\
\hline      
\multicolumn{5}{c}{c) Subgroup $G_2$}\\
\hline
Schedule        & $E(N^S_j)$ & $E(O^S_j)$ & ${\mbox{SD}(N^S_j)}$ & ${\mbox{SD}(O^S_j)}$ \\
\hline
Annual         & 5.18            & 5.98                & 2.13          & 3.47              \\
PRIAS          & 4.85            & 7.70                & 2.00          & 6.29        \\
Dyn. risk GR ($\mbox{F}_1$ score)       & 4.63            & 6.66                & 1.82          & 4.37              \\
Hybrid ($\mbox{F}_1$ score)       & 3.68            & 10.32                & 1.37          & 7.45              \\
Dyn. risk GR ($\kappa=0.95$) & 5.09 & 5.99 & 2.11 & 3.47\\
Med. GR time & 1.89             & 12.33               & 1.16          & 9.44              \\
Exp. GR time & 1.77            & 13.54               & 0.98          & 9.83              \\
\hline      
\multicolumn{5}{c}{d) Subgroup $G_3$}\\
\hline
Schedule        & $E(N^S_j)$ & $E(O^S_j)$ & ${\mbox{SD}(N^S_j)}$ & ${\mbox{SD}(O^S_j)}$ \\
\hline
Annual         & 6.20             & 6.02                & 1.76          & 3.46              \\
PRIAS          & 5.76             & 7.98                & 1.71         & 6.51        \\
Dyn. risk GR ($\mbox{F}_1$ score)       & 5.58            & 6.58                & 1.56          & 4.33              \\
Hybrid ($\mbox{F}_1$ score)       & 4.32            & 8.55                & 1.26          & 5.91              \\
Dyn. risk GR ($\kappa=0.95$) & 6.11 & 6.01 & 1.76 & 3.46\\
Med. GR time & 2.45            & 8.70                & 1.15          & 6.32              \\
Exp. GR time & 2.27            & 10.09               & 0.99          & 7.47              \\
\hline     
\end{tabular}
\end{table}

\clearpage

\subsection{Variation in Estimated Mean and Standard Deviation, of Number of Biopsies and Offset Across the 500 Simulations}
In this section we present figures related to the simulation study results discussed in Section \ref{sec: simulation_study} of main manuscript. The figures we present next are population specific, i.e. subgroup level differentiation is not done.

\begin{itemize}
  \item Variation in estimated mean across the 500 simulations, for number of biopsies and offset (months) for different methods is shown in Web Figure \ref{fig : nbMeanBoxPlot_all} and Web Figure \ref{fig : offsetMeanBoxPlot_all}.
  \item Variation in estimated standard deviation across the 500 simulations, for number of biopsies and offset (months) for different methods is shown in Web Figure \ref{fig : nbSDBoxPlot_all} and Web Figure \ref{fig : offsetSDBoxPlot_all}.
\end{itemize}

\begin{figure}[!htb]
\centerline{\includegraphics[width=\columnwidth]{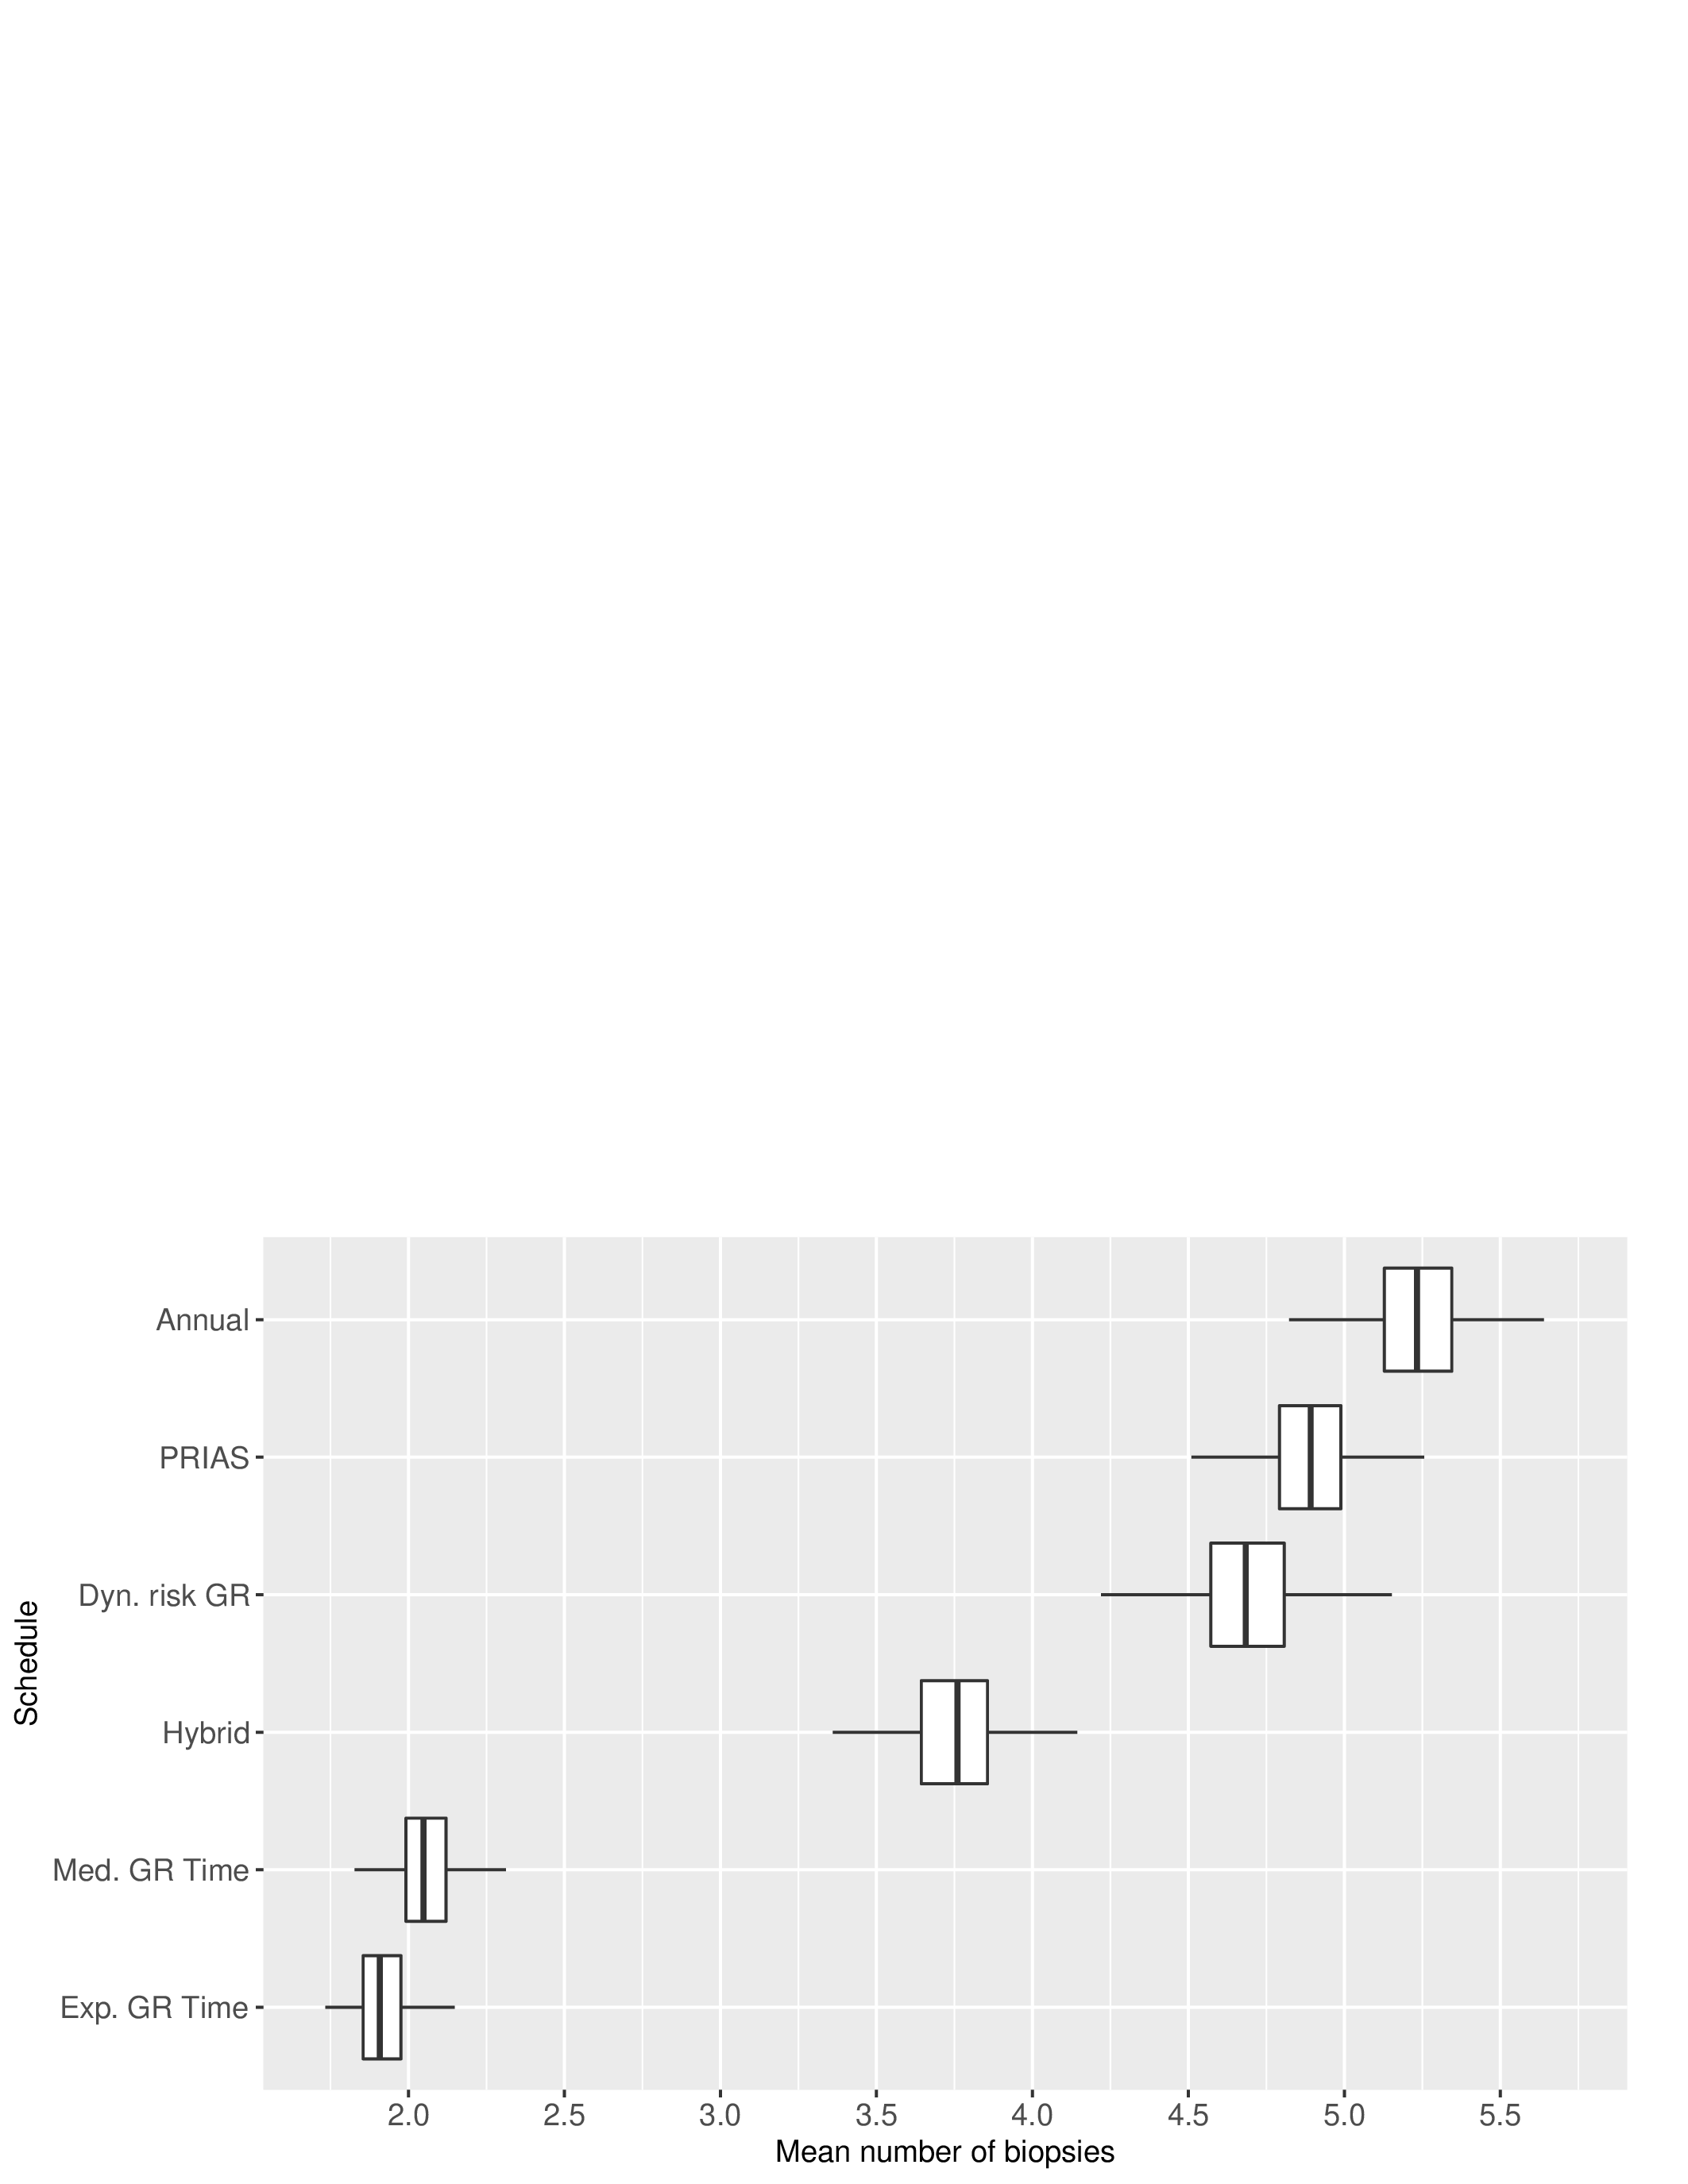}}
\caption{Boxplot showing variation in estimated mean number of biopsies across the 500 simulations, for different methods. Patients from all subgroups are considered.}
\label{fig : nbMeanBoxPlot_all}
\end{figure}

\begin{figure}[!htb]
\centerline{\includegraphics[width=\columnwidth]{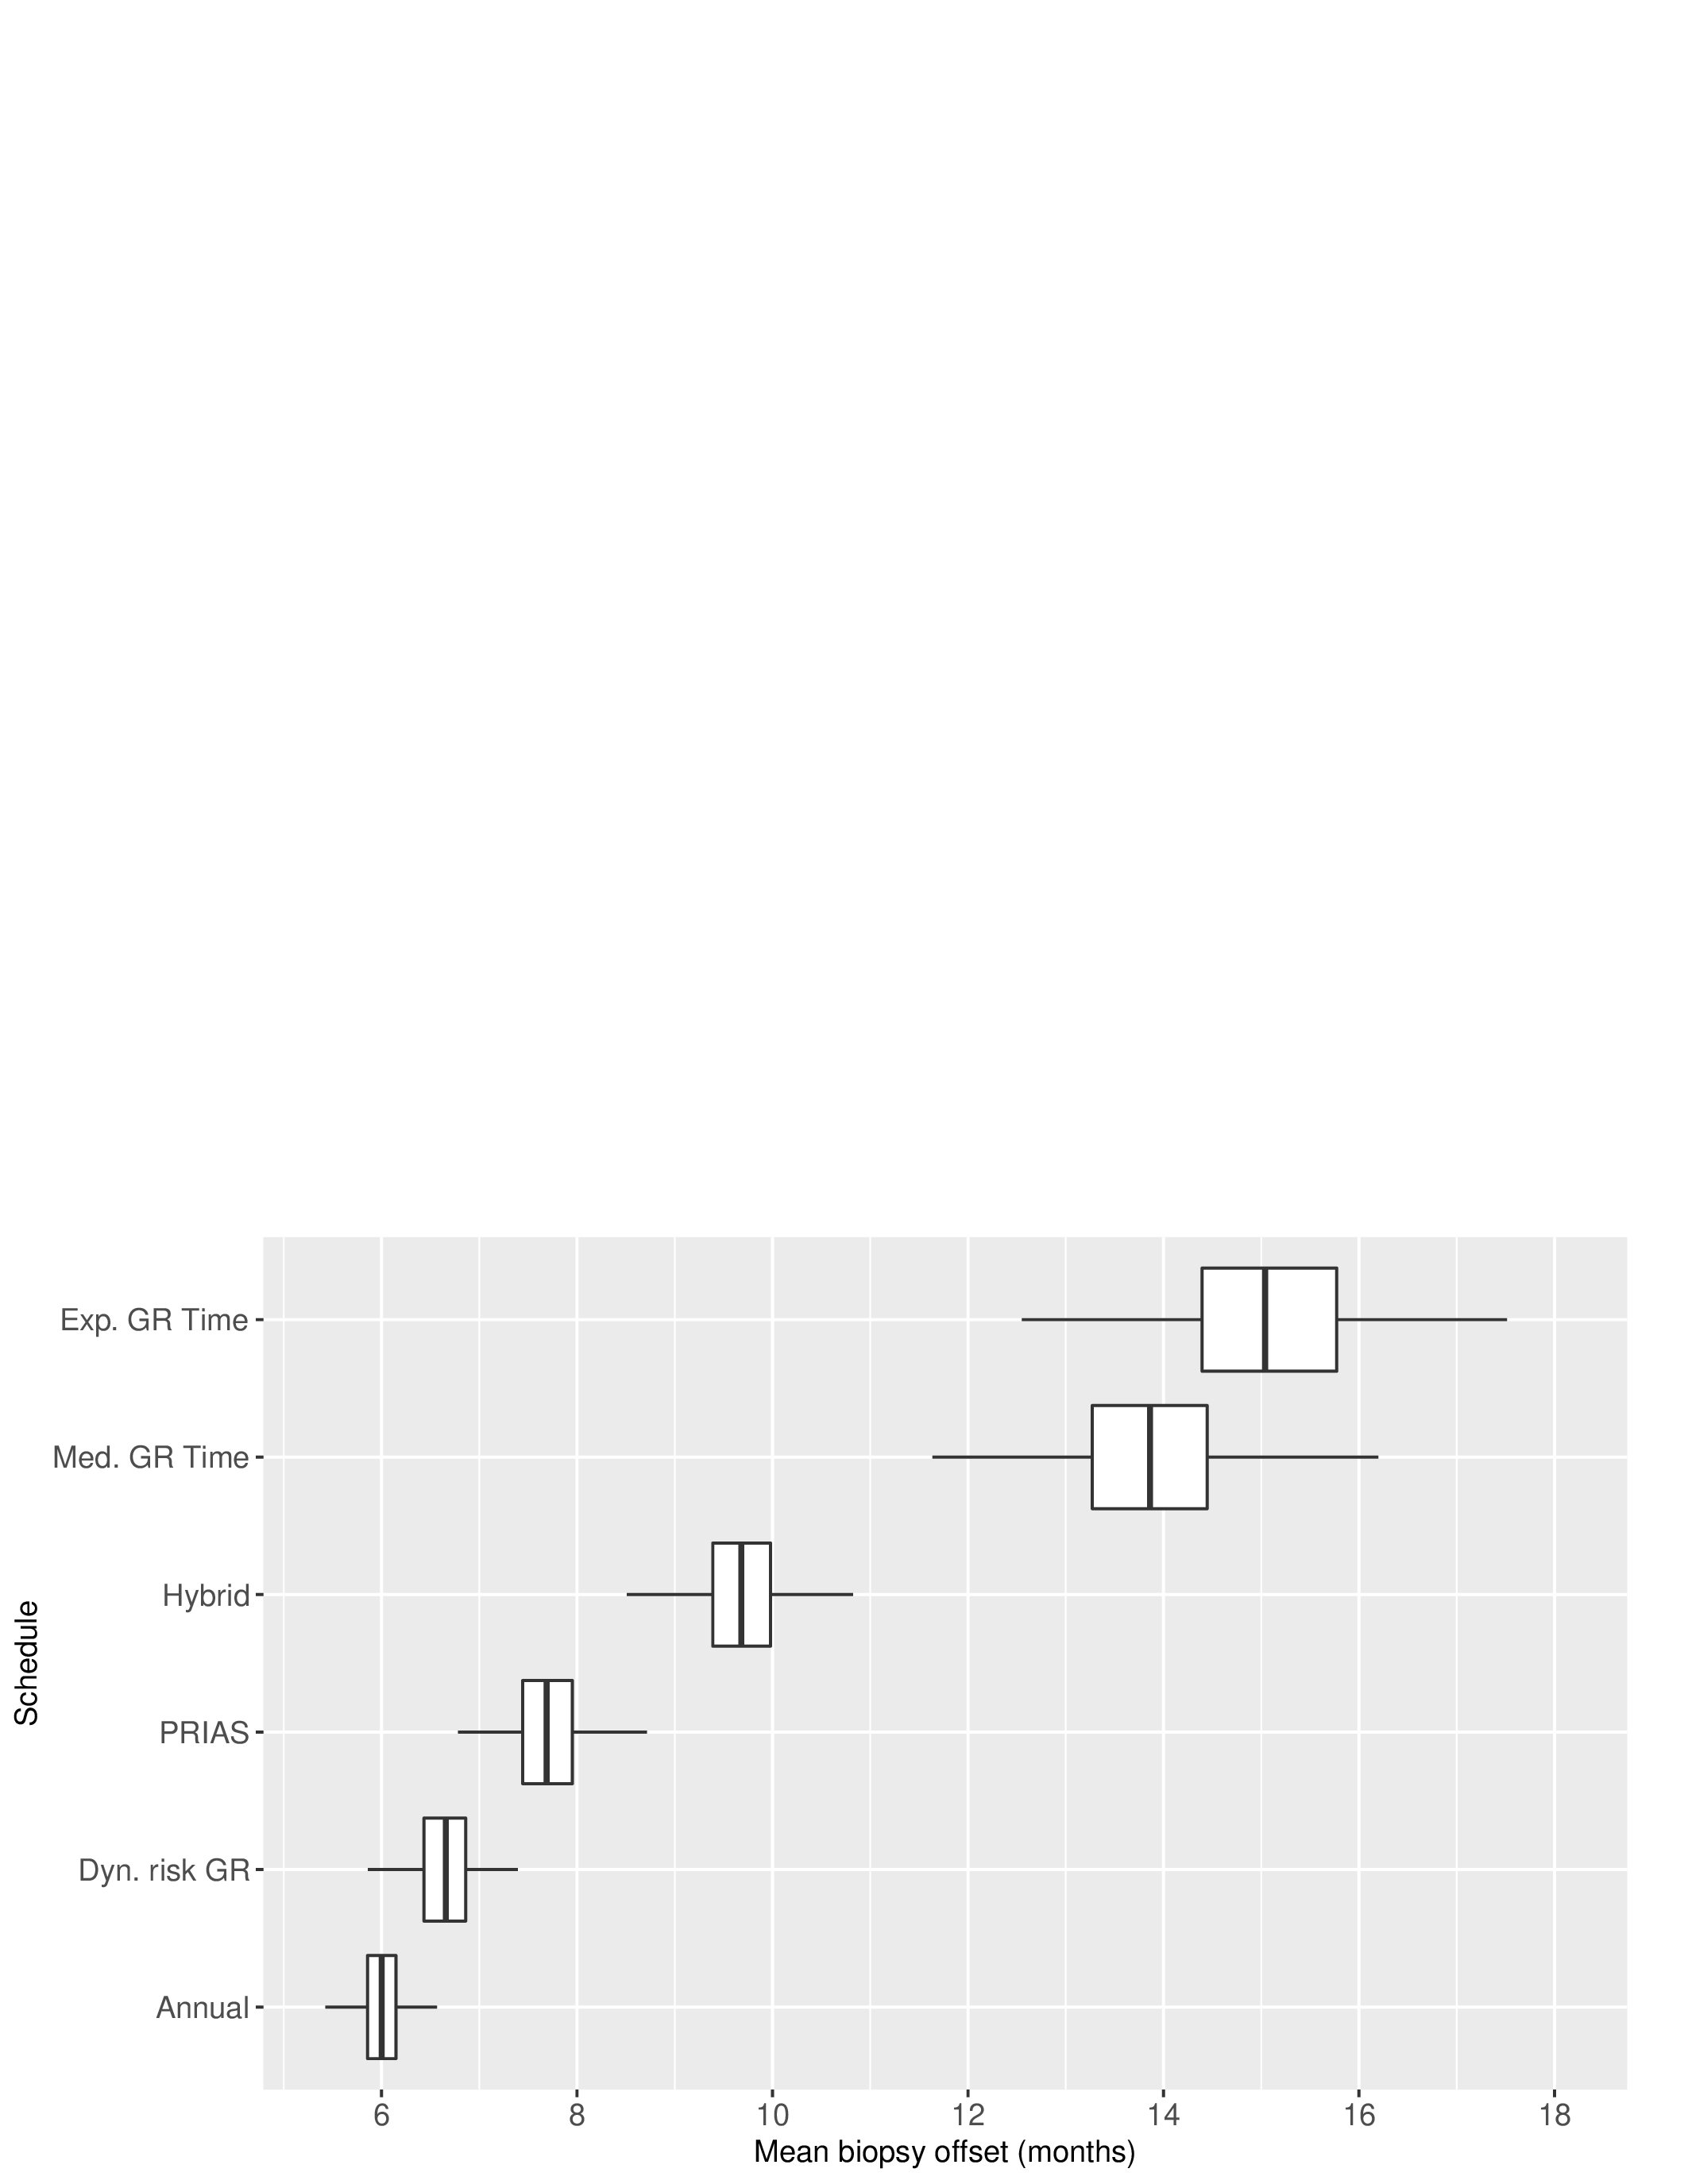}}
\caption{Boxplot showing variation in estimated mean of biopsy offset (months) across the 500 simulations, for different methods. Patients from all subgroups are considered.}
\label{fig : offsetMeanBoxPlot_all}
\end{figure}

\begin{figure}[!htb]
\centerline{\includegraphics[width=\columnwidth]{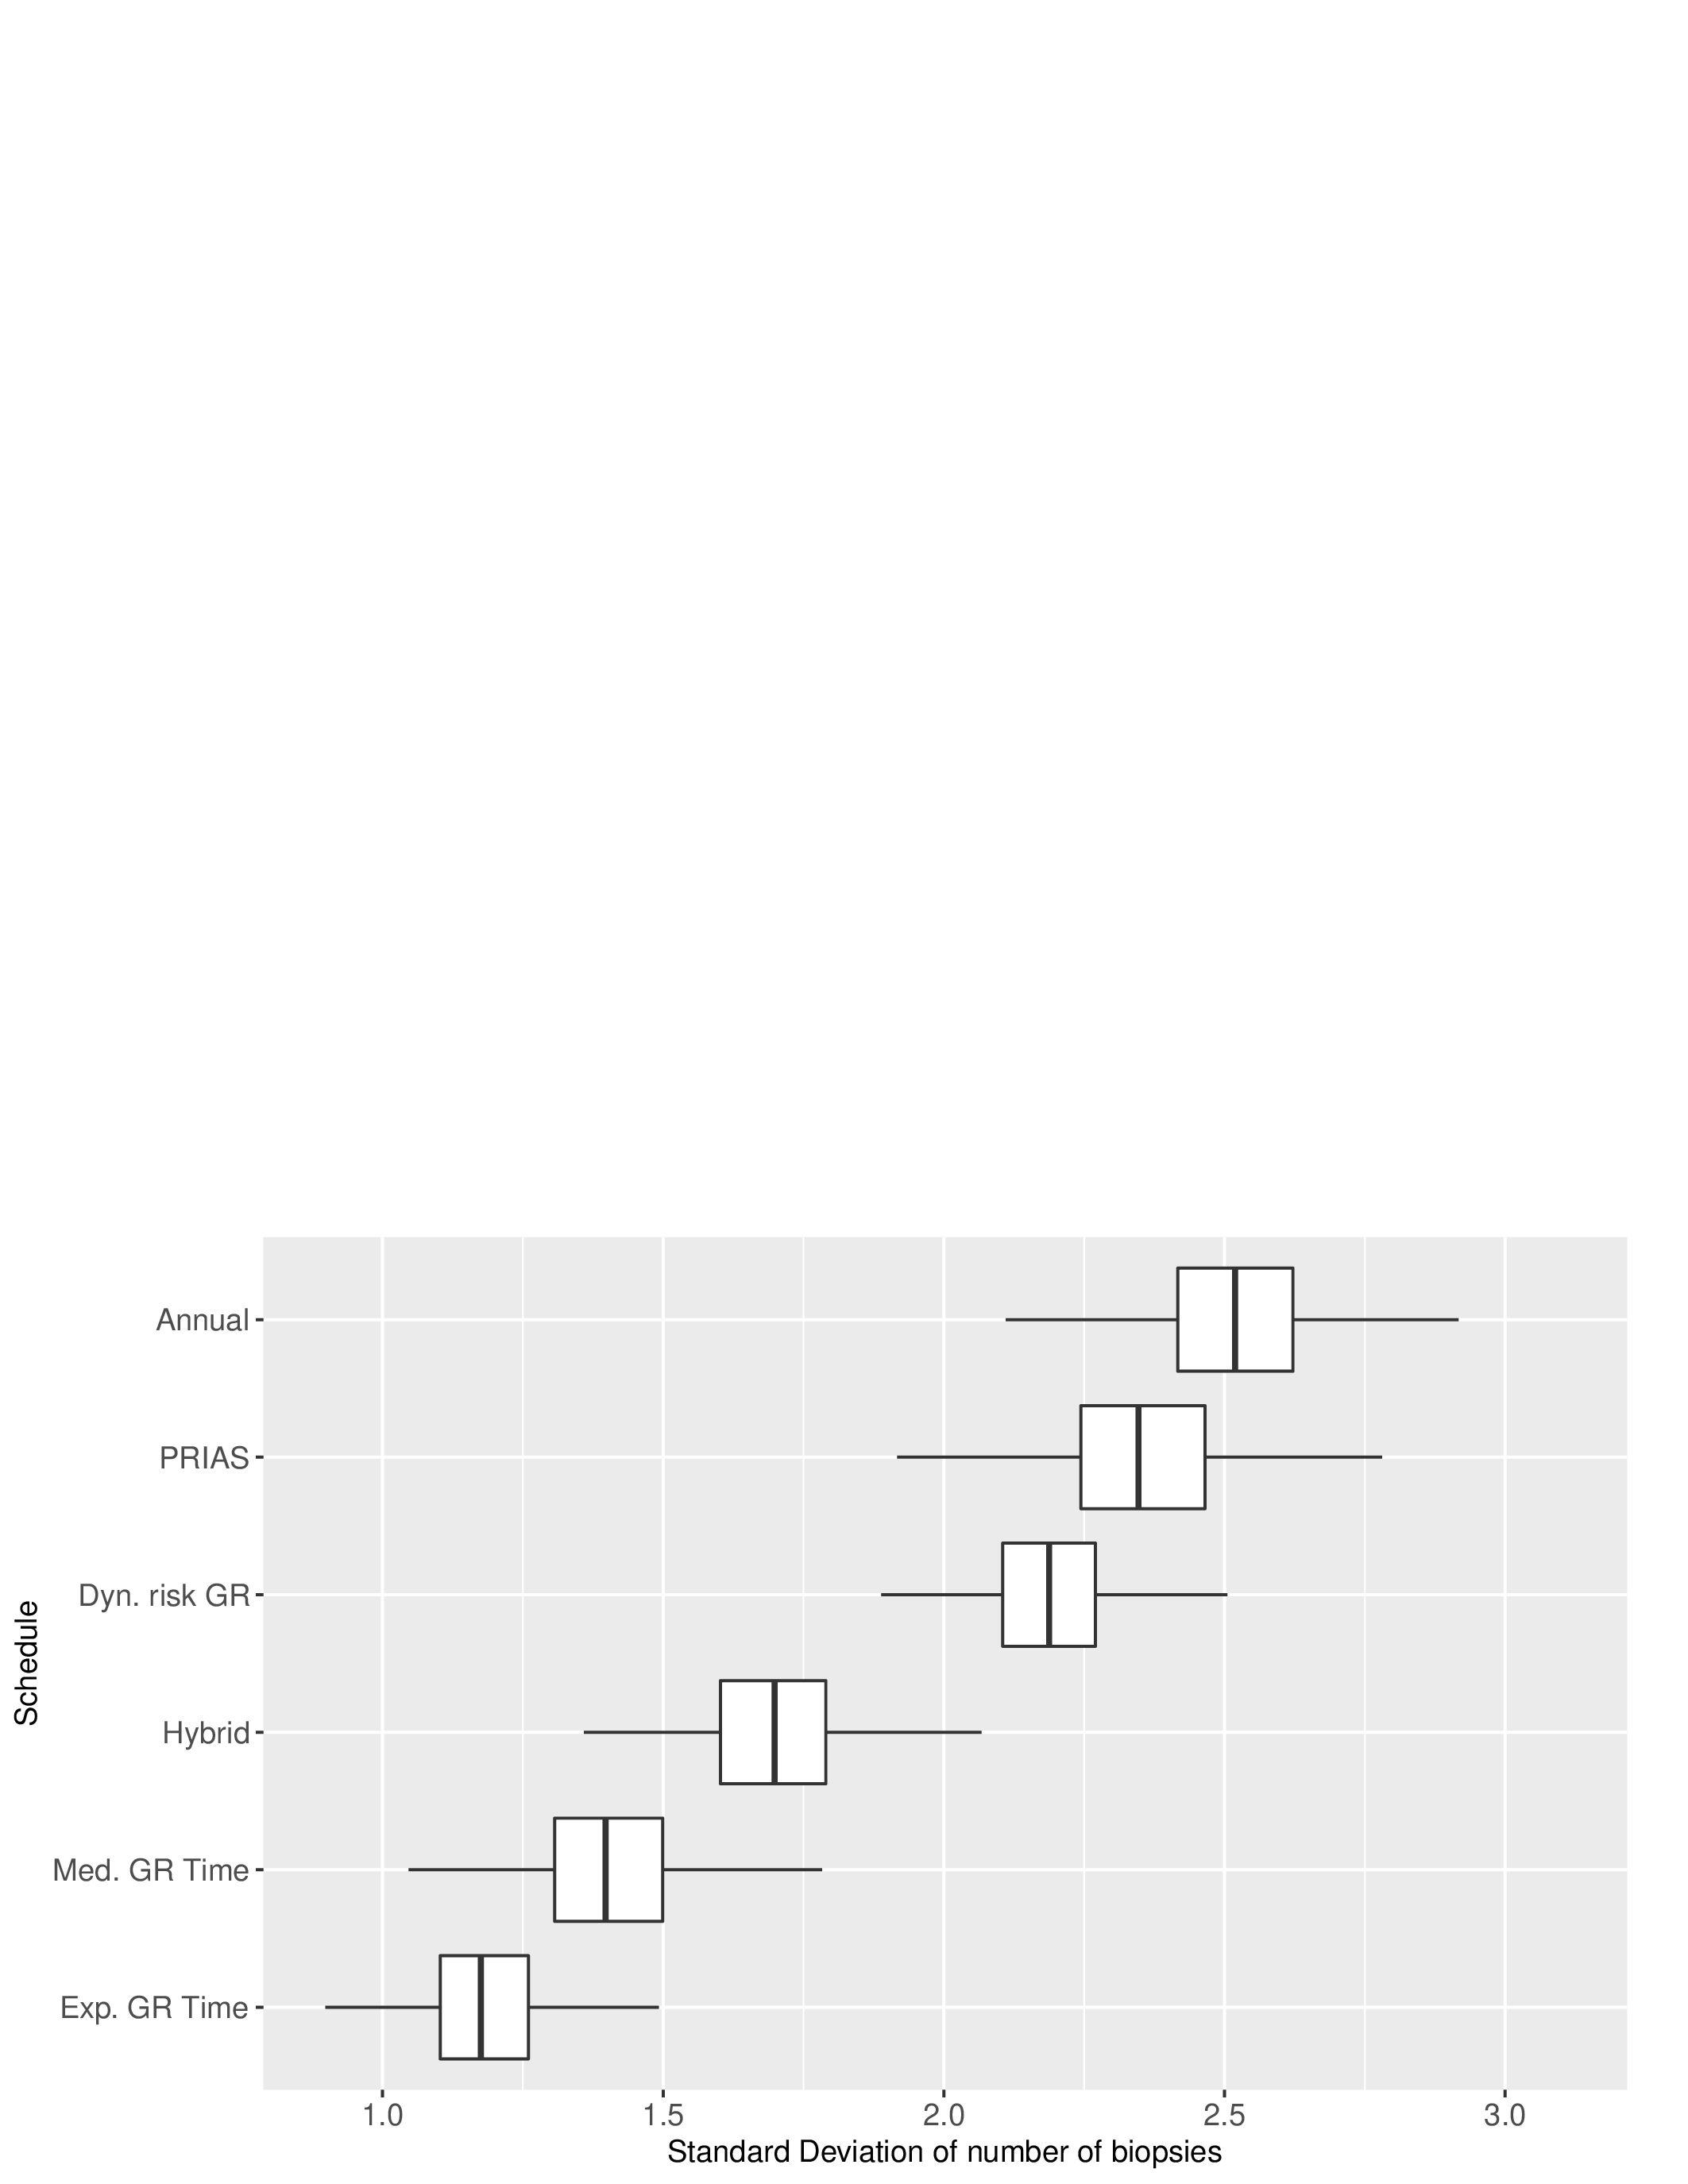}}
\caption{Boxplot showing variation in estimated standard deviation of number of biopsies across the 500 simulations, for different methods. Patients from all subgroups are considered.}
\label{fig : nbSDBoxPlot_all}
\end{figure}

\begin{figure}[!htb]
\centerline{\includegraphics[width=\columnwidth]{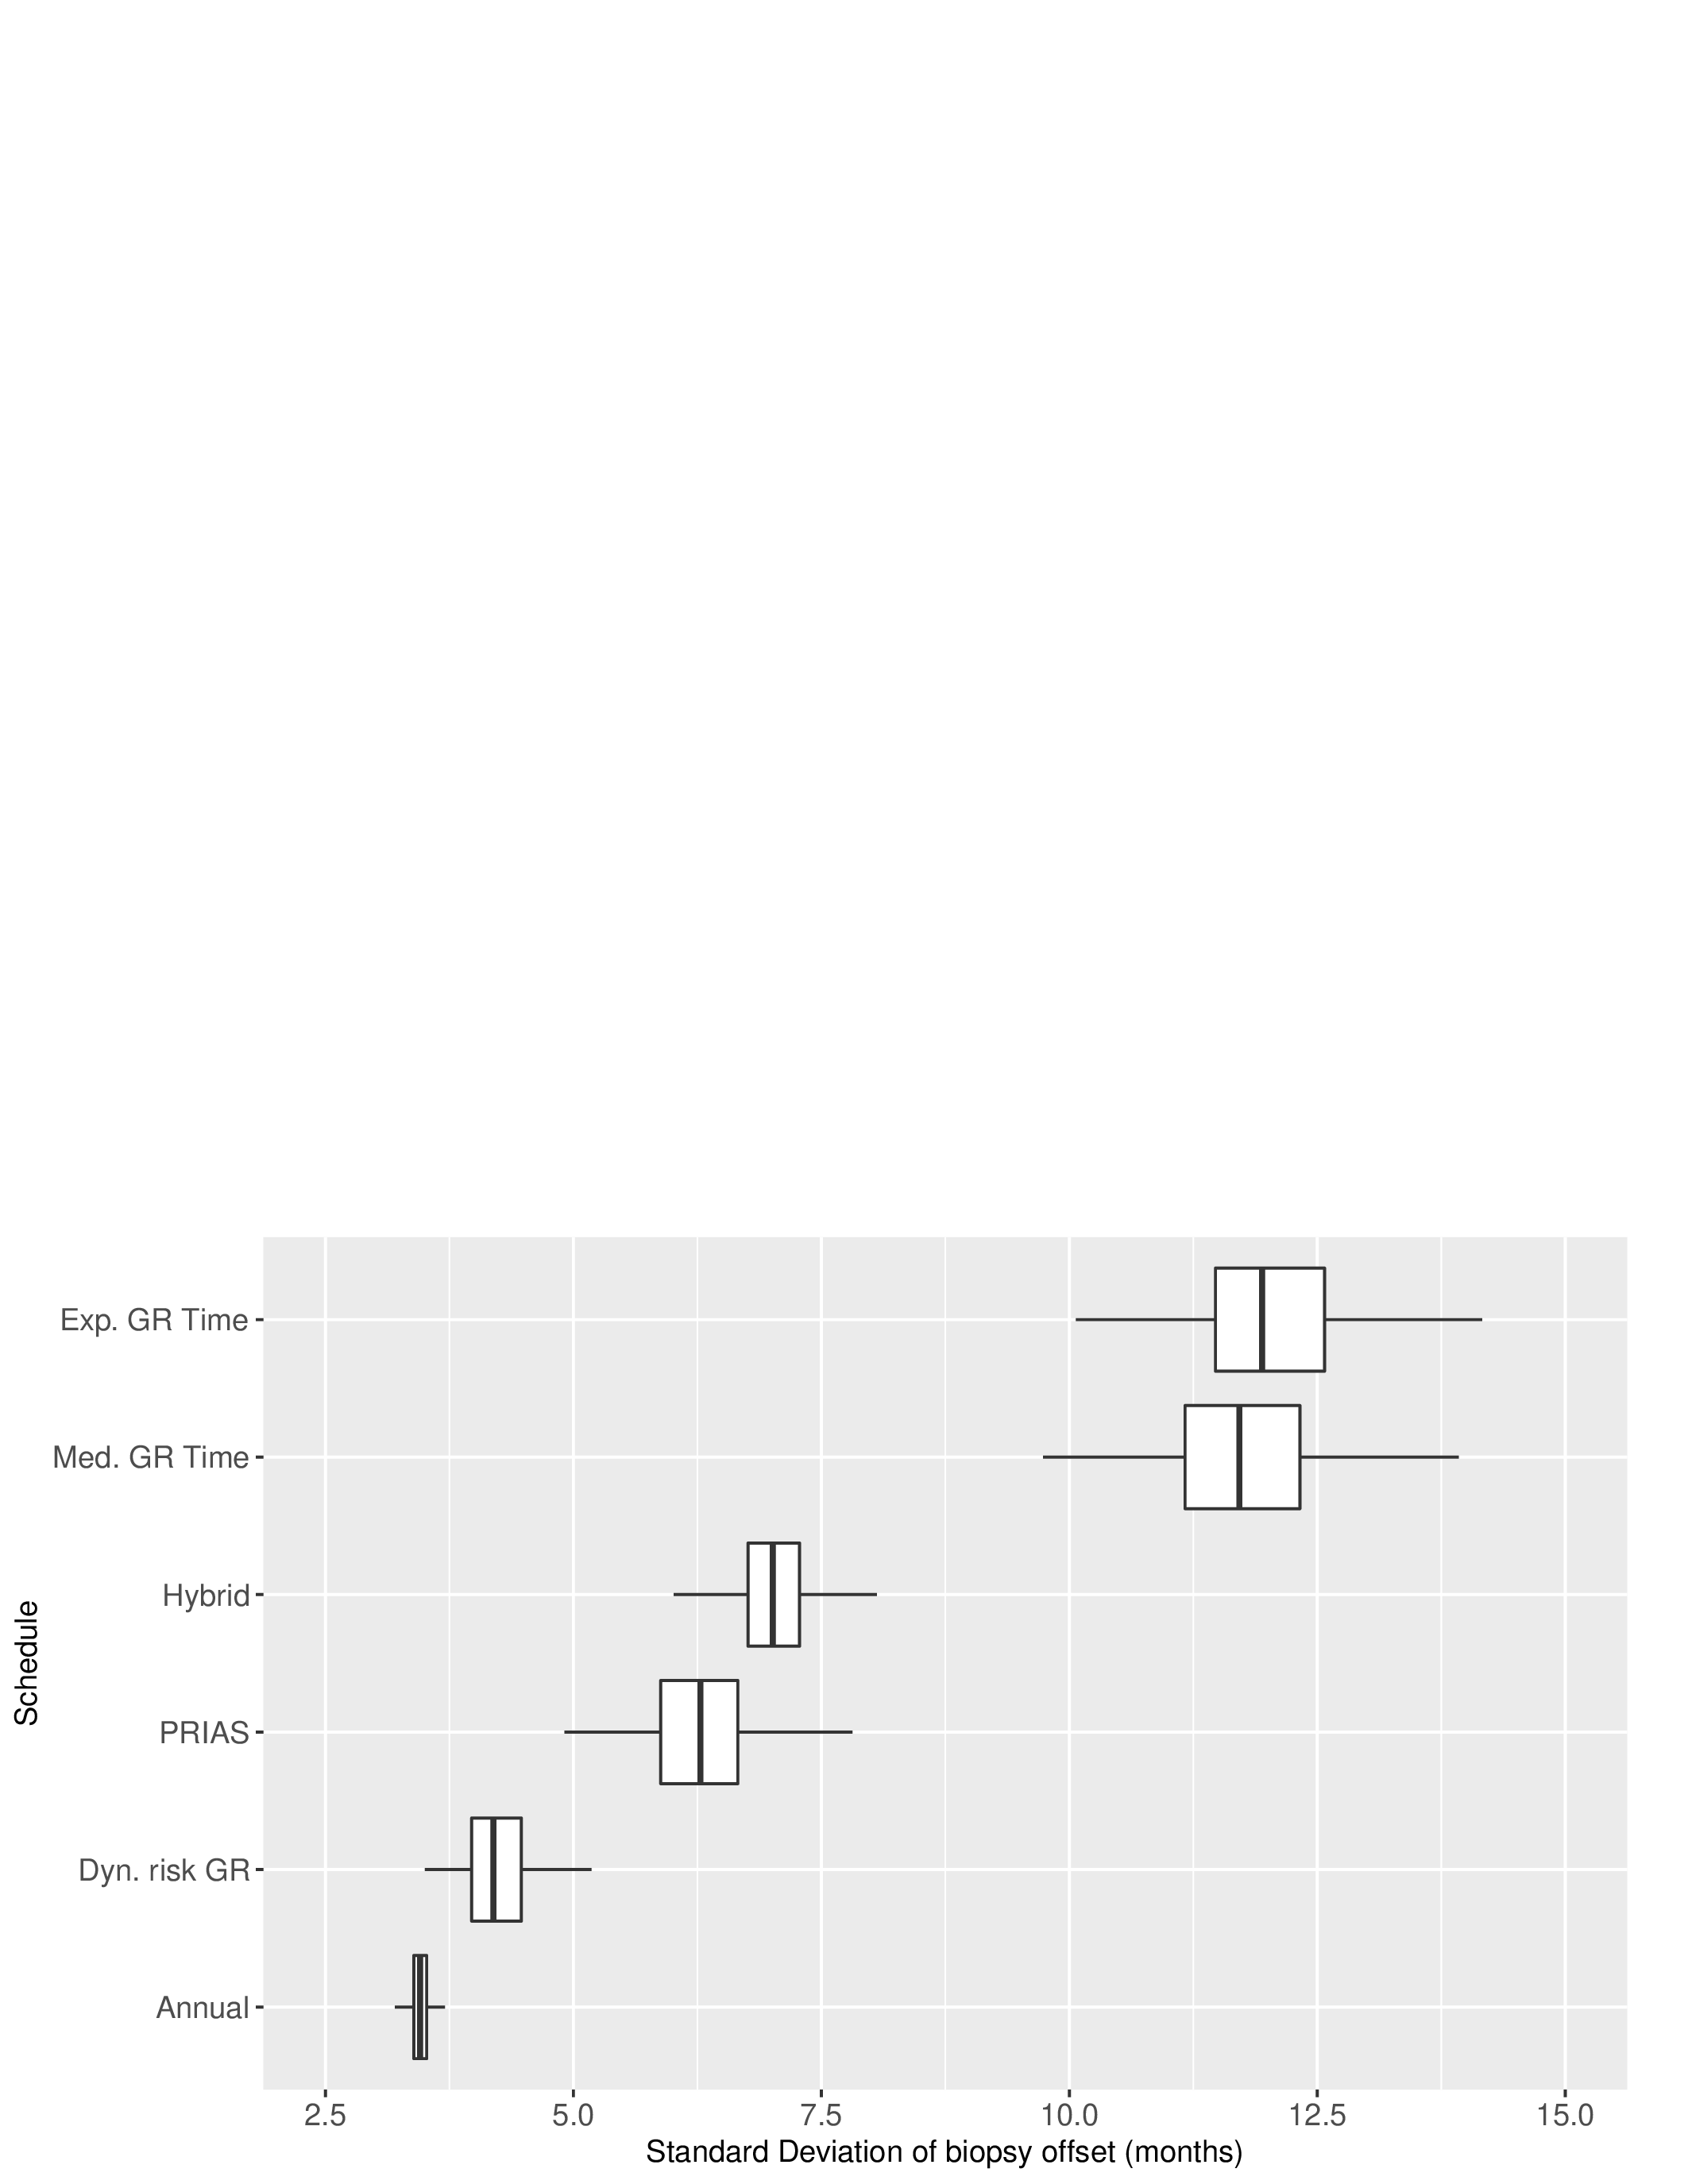}}
\caption{Boxplot showing variation in estimated standard deviation of biopsy offset (months) across the 500 simulations, for different methods. Patients from all subgroups are considered.}
\label{fig : offsetSDBoxPlot_all}
\end{figure}
