# Supplementary material for: Personalized Schedules for Surveillance of Low Risk Prostate Cancer Patients
Source: arXiv:1711.00285 source file (2017-11-01)
Supplement: Supplementary file 7 [file source_code.tex]

% !TEX root =  ../supplementary.tex
\section{Source code}
The source code for the joint model fitted to the PRIAS data set can be found at:\\
\url{https://goo.gl/phQkxG}\\
The source code for the simulation study can be found at:\\
\url{https://goo.gl/TpLTM8}\\
A README file explaining the usage of the code can be found at:\\
\url{https://goo.gl/h2pAep}.\\
